# Supplementary material for: Carrier Selectivity and Passivation at the Group V elemental 2D Material--Si Interface of a PV Device
Source: arXiv:2401.02648 ancillary file (2024-01-05)
Supplement: Supplementary file 1 [file supplement.pdf]

## Supplementary Information

### Carrier Selectivity and Passivation at the Group V elemental 2D Material–Si Interface of a PV Device

Gurudayal Behera,<sup>1</sup> K. R. Balasubramaniam,<sup>1,\*</sup> and Aftab Alam<sup>2,†</sup>

<sup>1</sup>*Department of Energy Science and Engineering, IIT Bombay, Powai, Mumbai 400076, India*

<sup>2</sup>*Department of Physics, Indian Institute of Technology, Bombay, Powai, Mumbai 400076, India*

Here, we provide further model structural data and their related data and related discussion to strengthen our message in the manuscript.

#### I. Crystal structures and surface formation energies of various possible configurations $\alpha$ -As/Si (111) interfacial surface slabs

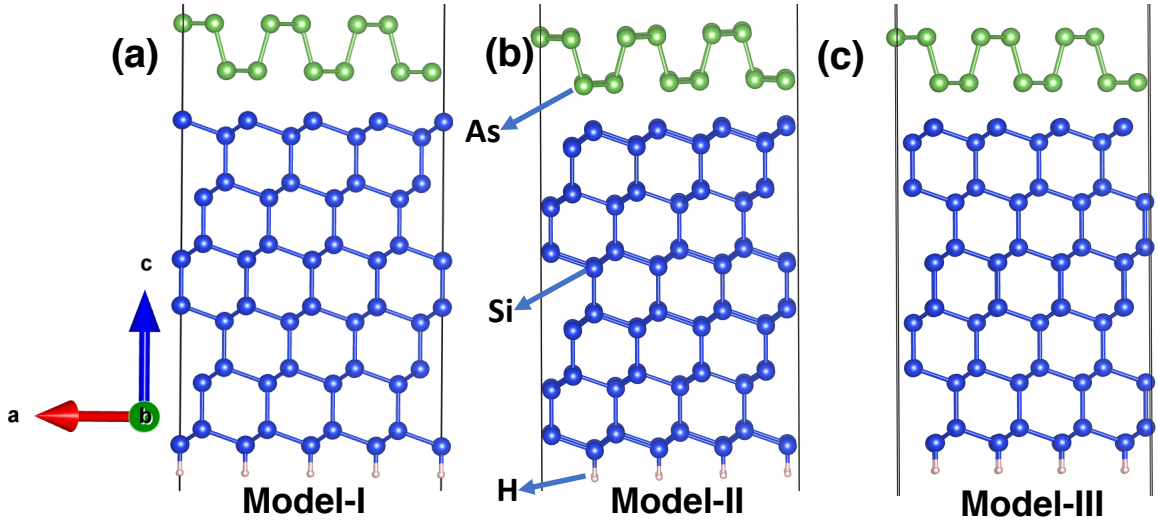

FIG. S1. Prototype crystal structure of various  $\alpha$ -As/Si(111):H. White, green, and blue spheres represent H, As, Si atoms, respectively.

TABLE S1. Formation energy for various models of  $\alpha$ -As/Si(111):H interface structures.

| Interface structure type | $E_{\text{form}}$ (eV/ $\text{\AA}^2$ )<br>$\alpha$ -As/Si:H |
|--------------------------|--------------------------------------------------------------|
| Model-I                  | 0.03                                                         |
| Model-II                 | 0.12                                                         |
| Model-III                | 0.08                                                         |

\* bala.ramanathan@iitb.ac.in

† aftab@iitb.ac.in

## II. Crystal structures and surface formation energies of various possible configurations $\beta$ -As/Sb/Bi with Si (111) surface slabs

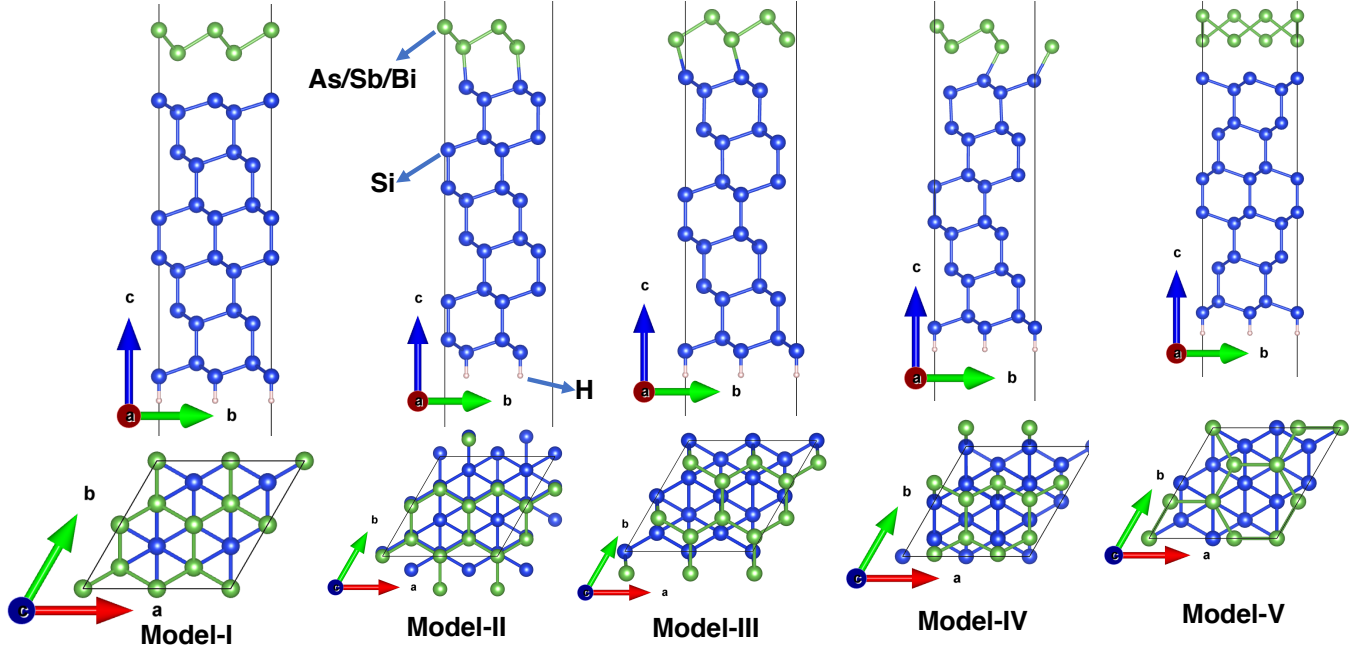

FIG. S2. Prototype crystal structure of various  $\beta$ -As/Si(111):H,  $\beta$ -Sb/Si(111):H, and  $\beta$ -Bi/Si(111):H interfacial surface slabs.

TABLE S2. Formation energy for various models of  $\beta$ -arsenene, antimonene and bismuthene with Si(111) heterostructures.

| Interface structure type | $E_{\text{form}}$ (eV/ $\text{\AA}^2$ )<br>$\beta$ -As/Si:H | $E_{\text{form}}$ (eV/ $\text{\AA}^2$ )<br>$\beta$ -Sb/Si:H | $E_{\text{form}}$ (eV/ $\text{\AA}^2$ )<br>$\beta$ -Bi/Si:H |
|--------------------------|-------------------------------------------------------------|-------------------------------------------------------------|-------------------------------------------------------------|
| Model-I                  | 0.08                                                        | 0.09                                                        | 0.06                                                        |
| Model-II                 | 0.03                                                        | 0.03                                                        | 0.02                                                        |
| Model-III                | 0.09                                                        | 0.12                                                        | 0.09                                                        |
| Model-IV                 | 0.13                                                        | 0.11                                                        | 0.14                                                        |
| Model-V                  | 0.22                                                        | 0.26                                                        | 0.32                                                        |

### III. Crystal structures and DOS plots for 2D monolayers and Si(100) heterostructures

Herein, we are presenting crystal structures and electronic properties of all the meta stable 2D monolayers/Si(100):H interfacial surface slabs. Figure S3 in depicts the crystal structures (before and after structural relaxation) along with their projected DOS plots. However, the other interface structures involving  $\alpha$ -As,  $\beta$ -Sb and  $\beta$ -Bi with Si(100) surface and their coresponding electronic structures are shown in Fig. S4. After structural optimization of the Si(100) based interfaces, a slight distortion in the Si layer at the interface region is observed in all the cases (see Fig. S3(b, e) and Fig S4). All the interfacial Si atoms are found to interact with As, Sb, and Bi in their respective interfaces, making the chemical bond between interfacial Si atoms and the group-V atoms. Expect for the  $\beta$ -Sb/Si:H interface (see Fig.S4 (d)), in all the other interfaces, Si atoms at the interface layer appear to form a Si-Si dimer with a bond length varying in between 2.40 Å to 2.46 Å. A similar type of Si dimers formation are also observed in  $\beta$ -MoO<sub>3</sub>/Si interface [1] and in the case of the WO<sub>3</sub>/Si interface reported by wang *et al.* [2]. The Si-Si bond length in the Si surface changes from 2.46 Å (near the interface) to 2.34 Å as we move away from the interface toward the bulk-like Si layers in all cases. This indicates significant surface reconstruction in the top layers and Si atoms exhibit bulk-like behavior as we move from top to bottom layers.

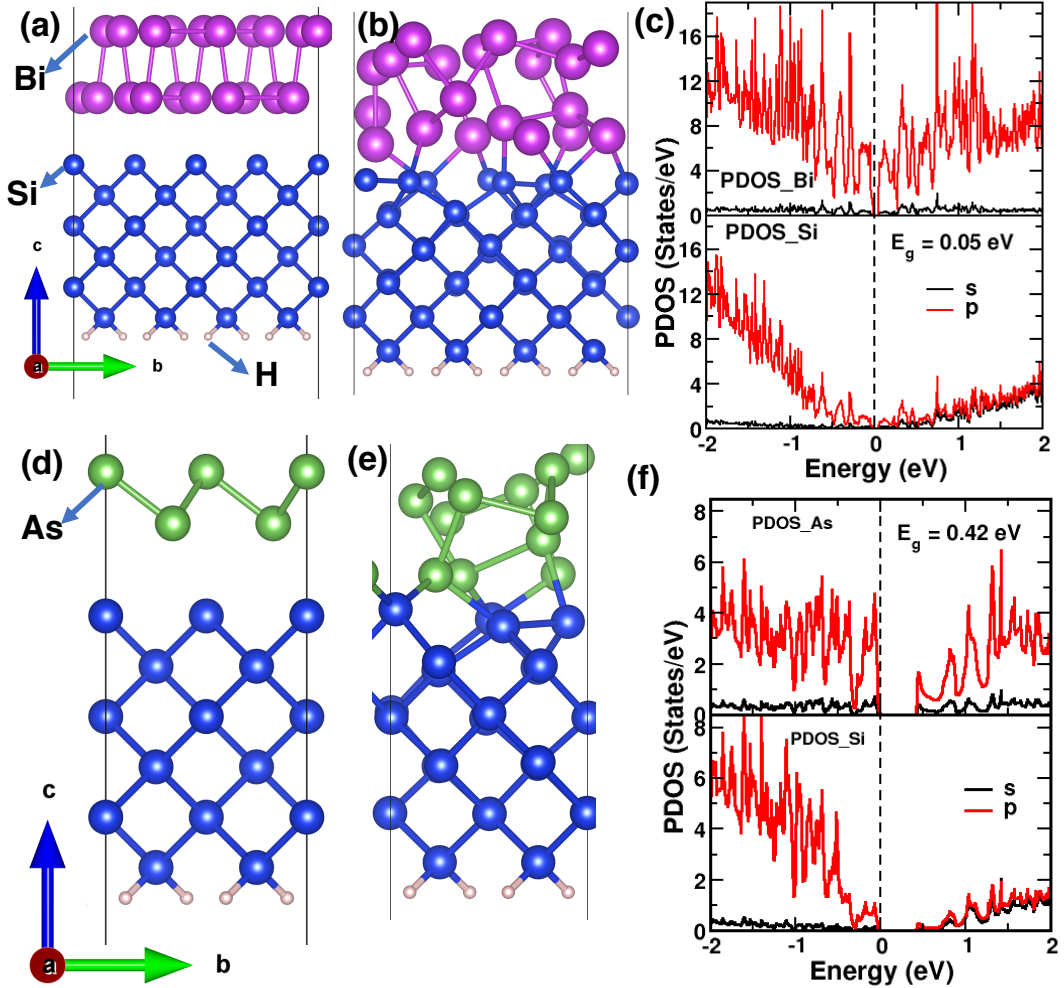

FIG. S3. Interfacial surface slab of  $\alpha$ -Bi/Si(100):H, and  $\beta$ -As/Si(100):H (a, d) before and (b, c) after ionic relaxation. White, green, magenta, and blue spheres represent H, As, Bi and Si atoms, respectively. (c, f) Orbital projected PDOS for  $\alpha$ -Bi/Si(100):H, and  $\beta$ -As/Si(100):H heterostructures, respectively.

Figure S3(c and f) shows the orbital projected DOS plots for the  $\alpha$ -Bi/Si(100), and  $\beta$ -As/Si(100) interfaces. The PDOS plot reveals that both the interface structures  $\alpha$ -Bi/Si and  $\beta$ -As/Si are semiconducting, indicating a band gap of 0.05 eV and 0.42 eV, respectively. The semiconducting nature of interfacial surface slabs suggests that  $\alpha$ -bismuthene and  $\beta$ -arsene monolayers can effectively saturate the Si dangling bonds and mimic the verisimilitude bulk character

of the Si surface. Therefore, it is reasonable to speculate that  $\alpha$ -bismuthene and  $\beta$ -arsenene are the best candidates for the passivating layer to Si surface in solar PV devices. In contrast, the other interfaces *i.e.*,  $\alpha$ -As/Si,  $\beta$ -Sb/Si(100), and  $\beta$ -Bi/Si(100) are found to be metallic in nature, as evident from their PDOS plots as shown in Fig. S4 (g, h, i) of SI. The major contributions of the electronic states at the  $E_f$  arise from As, Sb, and Bi atoms. The individual contribution of each Si layer to the total DOS, the PDOS of each Si layer for all the metallic interfaces are checked. It observed that the electronic states at/near  $E_f$  for each layer of Si atoms decrease as we move from the top to the bottom in the Si slab.

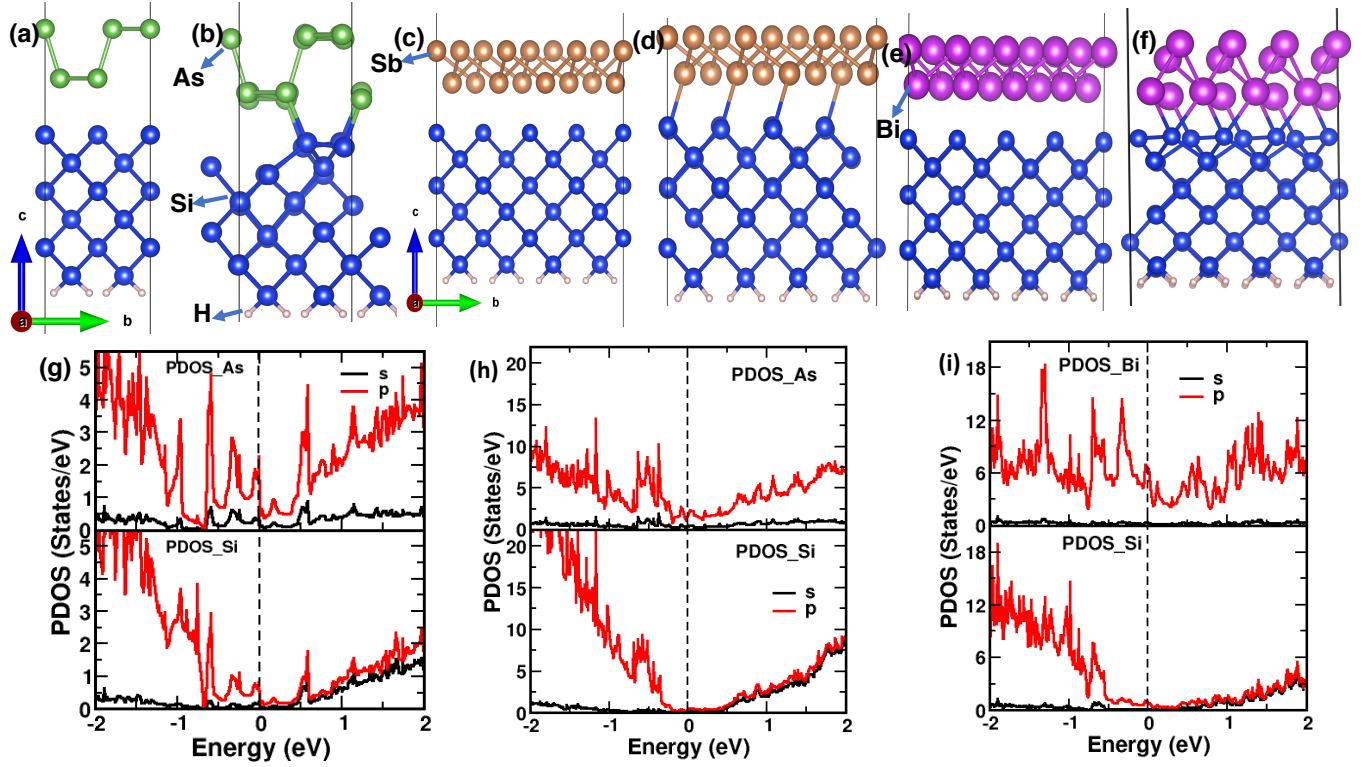

FIG. S4. Heterostructures of  $\alpha$ -As/Si(100):H,  $\beta$ -Sb/Si(100):H, and  $\beta$ -Bi/Si(100):H (a, c, e) before ionic relaxation (b, d, f) after relaxation. White, green, brown, magenta and blue spheres represent H, As, Sb, Bi, and Si atoms, respectively. (g, h, i) Orbital projected DOS for s-orbital (black color) and p-orbitals (red color) of As, Sb, Bi and Si atoms for  $\alpha$ -As/Si(100):H,  $\beta$ -Sb/Si(100):H, and  $\beta$ -Bi/Si(100):H surface slabs, respectively.

- 
- [1] G. Behera, Vikram, A. Kumar, K. Balasubramaniam, and A. Alam, First-Principles Study of the Surface Passivation Effect in the Si/MoO<sub>x</sub> Interface, J. Phys. Chem. C **125**, 11513 (2021).
  - [2] W. Wang, S. Chen, P.-X. Yang, C.-G. Duan, and L.-W. Wang, Si:WO<sub>3</sub> heterostructure for Z-scheme water splitting: an AB initio study, J. of Mater. Chem. A **1**, 1078 (2013).
